# Supplementary material for: LightLM: A Lightweight Deep and Narrow Language Model for Generative Recommendation
Source: arXiv:2310.17488 source file (2023-10-30)
Supplement: Supplementary file 1 [file appendix.tex]

\appendix
\section{Appendix} \label{sec:appendix}

\subsection{Dataset} \label{sec:dataset}
\input{tabs/data_info}
% \subsection{More Efficiency Results of LightP5} \label{sec:more_efficiency}
